# Supplementary material for: Post-Processed Posteriors for Sparse Covariances and Its Application to Global Minimum Variance Portfolio
Source: arXiv:2108.09462 source file (2021-08-21)
Supplement: Supplementary file 2 [file supplementary_material.pdf]

# Supplementary material of “Post-Processed Posteriors for Sparse Covariances and Its Application to Global Minimum Variance Portfolio”

Kwangmin Lee<sup>1</sup> and Jaeyong Lee<sup>1</sup>

<sup>1</sup>*Department of Statistics, Seoul National University*

August 6, 2021

In the supplementary material, we provide the proofs of lemmas and theorems in the main paper.

We let  $A_{\{i,j\} \times \{i,j\}}$  denote  $2 \times 2$  sub-matrix of  $A$  with  $i, j$  row and column for a matrix  $A$ . For a  $p \times p$  symmetric matrix  $A$ , let  $\text{diag}(A)$  be a  $p \times p$  diagonal matrix in which diagonal elements are equal to those of  $A$ . We also let  $\text{diag}^c(A) = A - \text{diag}(A)$ .

## S1 Proof of Theorem 2.1 and Related Lemma

In this section, we prove Theorem 2.1. First, we present Lemma S1.1 which gives an inequality for thresholded covariances.

**Lemma S1.1.** *Let  $n, p$  and  $r$  be positive integers and  $\gamma$  be a positive real number. Suppose  $\Sigma_0 = (\sigma_{0,ij})_{1 \leq i,j \leq p} \in \mathcal{G}_q(c_{n,p}, M_0, M_1)$ . There exist a positive constant  $C$  such that*

$$\begin{aligned} \|H_\gamma(\Sigma) - \Sigma_0\|_1^r &\leq 2^{r-1} \|D\|_1^r + 4^{r-1} \left\{ 4C c_{n,p} \left( \frac{\log p}{n} \right)^{(1-q)/2} \right\}^r + \left\{ 4\gamma \left( \frac{\log p}{n} \right)^{1/2} \right\}^r, \\ \|\text{diag}^c\{H_\gamma(\Sigma) - \Sigma_0\}\|_1^r &\leq 2^{r-1} \|D\|_1^r + 2^{r-1} \left\{ 4C c_{n,p} \left( \frac{\log p}{n} \right)^{(1-q)/2} \right\}^r, \end{aligned}$$

where  $D = (d_{ij})_{1 \leq i,j \leq p}$ ,  $d_{ij} = (H_\gamma(\Sigma))_{ij} - \sigma_{0,ij} I(A_{ij}^c)$ , and

$$A_{ij} = \left\{ |(H_\gamma(\Sigma))_{ij} - \sigma_{0,ij}| \leq 4 \min \left\{ |\sigma_{0,ij}|, \gamma \sqrt{\frac{\log p}{n}} \right\} \right\}.$$

*Proof.* We have

$$\begin{aligned}
\|H_\gamma(\Sigma) - \Sigma_0\|_1^r &\leq 2^{r-1}\|D\|_1^r + 2^{r-1}\|\{(H_\gamma(\Sigma)_{ij} - \sigma_{0,ij})I(A_{ij})\}_{1 \leq i,j \leq p}\|_1^r \\
&\leq 2^{r-1}\|D\|_1^r + 4^{r-1}[\sup_j \sum_{i \neq j} |(H_\gamma(\Sigma)_{ij} - \sigma_{0,ij})I(A_{ij})|^r + 4^{r-1}\{\sup_j |(H_\gamma(\Sigma)_{jj} - \sigma_{0,jj})I(A_{jj})|\}^r] \\
&\leq 2^{r-1}\|D\|_1^r + 4^{r-1}\left[\sup_j \sum_{i \neq j} 4 \min\left\{|\sigma_{0,ij}|, \gamma\left(\frac{\log p}{n}\right)^{1/2}\right\}\right]^r + 4^{r-1}\left\{4\gamma\left(\frac{\log p}{n}\right)^{1/2}\right\}^r,
\end{aligned}$$

where the third inequality is satisfied by the definition of  $A_{ij}$ . Inequality (51) in the proof of Theorem 3 in Cai et al. (2012) gives

$$\sum_{i \neq j} \min\left\{|\sigma_{0,ij}|, \gamma\left(\frac{\log p}{n}\right)^{1/2}\right\} \leq Cc_{n,p}\left(\frac{\log p}{n}\right)^{(1-q)/2},$$

for a positive constant  $C$ . Thus, we get

$$\|H_\gamma(\Sigma) - \Sigma_0\|_1^r \leq 2^{r-1}\|D\|_1^r + 4^{r-1}\left\{4Cc_{n,p}\left(\frac{\log p}{n}\right)^{(1-q)/2}\right\}^r + 4^{r-1}\left\{4\gamma\left(\frac{\log p}{n}\right)^{1/2}\right\}^r.$$

Likewise, we have

$$\begin{aligned}
\|diag^c\{H_\gamma(\Sigma) - \Sigma_0\}\|_1^r &\leq 2^{r-1}\|diag^c(D)\|_1^r + 2^{r-1}\|\{(H_\gamma(\Sigma)_{ij} - \sigma_{0,ij})I(A_{ij})\}_{1 \leq i,j \leq p}\|_1^r \\
&\leq 2^{r-1}\|D\|_1^r + 2^{r-1}[\sup_j \sum_{i \neq j} |(H_\gamma(\Sigma)_{ij} - \sigma_{0,ij})I(A_{ij})|^r] \\
&\leq 2^{r-1}\|D\|_1^r + 2^{r-1}\left\{4Cc_{n,p}\left(\frac{\log p}{n}\right)^{(1-q)/2}\right\}^r.
\end{aligned}$$

□

**Lemma S1.2.** Suppose  $\Sigma \in \mathcal{G}_q(c_{n,p}, M_0, M_1)$ . If  $x < 4\|\Sigma_0\|$  and  $(\nu_n - 2p) \vee \|A\| = o(n)$ , then there exist positive constants  $C$  and  $\lambda$  such that

$$E_{\Sigma_0}\{P^{\pi^i}(|\sigma_{ij} - \sigma_{0,ij}| \geq x \mid \mathbb{X}_n)\} \leq C(\exp(-\lambda n) + \exp(-\lambda nx^2)),$$

for arbitrary  $i, j \in [p]$ .

*Proof.* Since  $[\Sigma_{\{i,j\} \times \{i,j\}} \mid \mathbb{X}_n] \sim IW_2(n + \nu_n - 2p + 4, A_{\{i,j\} \times \{i,j\}} + nS_{\{i,j\} \times \{i,j\}})$  (Press; 2012, Theorem 5.2.3), Lemma 6.2 in the supplementary material of Lee et al. (2021) gives

$$\begin{aligned}
&E_{\Sigma_0}\{P^{\pi^i}(|\sigma_{ij} - \sigma_{0,ij}| \geq x \mid \mathbb{X}_n)\} \\
&\leq E_{\Sigma_0}\{P^{\pi^i}(\|\Sigma_{\{i,j\} \times \{i,j\}} - (\Sigma_0)_{\{i,j\} \times \{i,j\}}\|_2 \geq x \mid \mathbb{X}_n)\} \\
&\leq C\{\exp(-\lambda n) + \exp(-\lambda nx^2)\},
\end{aligned}$$

for some positive constants  $C$  and  $\lambda$ .

□

**Lemma S1.3.** Suppose the same notations of Lemma S1.1. If  $(\nu_n - 2p) \vee \|A\| \vee \log p = o(n)$  and  $\gamma$  is a sufficiently large constant, then there exists a positive constant  $C$  such that

$$E\{E^{\pi^i}(\|D\|_1^2 \mid \mathbb{X}_n)\} = \frac{C}{n},$$

for all sufficiently large  $n$ .

*Proof.* We have

$$\begin{aligned} \|D\|_1^2 &\leq p \sum_{ij} d_{ij}^2 \\ &= p \sum_{ij} (H_\gamma(\Sigma)_{ij} - \sigma_{0,ij})^2 I(A_{ij}^c) \{I(|\sigma_{ij}| \geq \gamma(\log p/n)^{1/2}) + I(|\sigma_{ij}| < \gamma(\log p/n)^{1/2})\} \\ &\leq p \sum_{ij} (\sigma_{ij} - \sigma_{0,ij})^2 I(A_{ij}^c) I(|\sigma_{ij}| \geq \gamma(\log p/n)^{1/2}) \\ &\quad + p \sum_{ij} \sigma_{0,ij}^2 I(A_{ij}^c) I(|\sigma_{ij}| < \gamma(\log p/n)^{1/2}), \end{aligned}$$

where  $\sigma_{ij}$  is the  $(i, j)$  element of  $\Sigma$ . We also have

$$\begin{aligned} I(A_{ij}^c) I(|\sigma_{ij}| \geq \gamma(\log p/n)^{1/2}) &= I(A_{ij}^c) I(|\sigma_{ij}| \geq \gamma(\log p/n)^{1/2}) I(|\sigma_{0,ij}| < \frac{\gamma}{2} \left(\frac{\log p}{n}\right)^{1/2}) \\ &\quad + I(A_{ij}^c) I(|\sigma_{ij}| \geq \gamma(\log p/n)^{1/2}) I(|\sigma_{0,ij}| \geq \frac{\gamma}{2} \left(\frac{\log p}{n}\right)^{1/2}) \\ &\leq I(|\sigma_{ij}| \geq \gamma(\log p/n)^{1/2}) I(|\sigma_{0,ij}| < \frac{\gamma}{2} \left(\frac{\log p}{n}\right)^{1/2}) \\ &\quad + I(|\sigma_{ij} - \sigma_{0,ij}| > 4 \min\left\{|\sigma_{0,ij}|, \gamma \sqrt{\frac{\log p}{n}}\right\}) I(|\sigma_{0,ij}| \geq \frac{\gamma}{2} \left(\frac{\log p}{n}\right)^{1/2}) \\ &\leq I(|\sigma_{ij}| \geq \gamma(\log p/n)^{1/2}) I(|\sigma_{0,ij}| < \frac{\gamma}{2} \left(\frac{\log p}{n}\right)^{1/2}) \\ &\quad + I(|\sigma_{ij} - \sigma_{0,ij}| > 2\gamma(\log p/n)^{1/2}) \\ &\leq I(|\sigma_{ij}| - |\sigma_{0,ij}| \geq \frac{\gamma}{2} \left(\frac{\log p}{n}\right)^{1/2}) + I(|\sigma_{ij} - \sigma_{0,ij}| > 2\gamma(\log p/n)^{1/2}) \\ &\leq I(|\sigma_{ij} - \sigma_{0,ij}| \geq \frac{\gamma}{2} \left(\frac{\log p}{n}\right)^{1/2}), \end{aligned} \tag{S1}$$

where the first inequality is satisfied by the definitions of  $A_{ij}$  and  $H_\gamma(\Sigma)$ . Next, we have

$$\begin{aligned} I(A_{ij}^c) I(|\sigma_{ij}| < \gamma(\log p/n)^{1/2}) &= I(|\sigma_{ij}| < \gamma(\log p/n)^{1/2}) I(|\sigma_{0,ij}| > 4 \min\left\{|\sigma_{0,ij}|, \gamma \sqrt{\frac{\log p}{n}}\right\}) \\ &\leq I(|\sigma_{0,ij}| - |\sigma_{ij} - \sigma_{0,ij}| \leq \gamma(\log p/n)^{1/2}) I(|\sigma_{0,ij}| > 4\gamma \sqrt{\frac{\log p}{n}}) \\ &\leq I(|\sigma_{ij} - \sigma_{0,ij}| \geq 3|\sigma_{0,ij}|/4) I(|\sigma_{0,ij}| > 4\gamma \sqrt{\frac{\log p}{n}}). \end{aligned} \tag{S2}$$

Using the inequalities (S1) and (S2), we get

$$E_{\Sigma_0}\{E^{\pi^i}(\|D\|_1^2 \mid \mathbb{X}_n)\} \leq p \sum_{ij} E\{E^{\pi^i}((\sigma_{ij} - \sigma_{0,ij})^2 I(|\sigma_{ij} - \sigma_{0,ij}| \geq \frac{\gamma}{2} \left(\frac{\log p}{n}\right)^{1/2}) \mid \mathbb{X}_n)\} \tag{S3}$$

$$+ p \sum_{ij} E\{E^{\pi^i}(\sigma_{0,ij}^2 I(|\sigma_{ij} - \sigma_{0,ij}| \geq \frac{3}{4} |\sigma_{0,ij}|) I(|\sigma_{0,ij}| > 4\gamma \sqrt{\frac{\log p}{n}}) \mid \mathbb{X}_n)\} \tag{S4}$$

For the upper bound of (S3), we have

$$(S3) \leq p^3 \sup_{ij} E_{\Sigma_0} \{E^{\pi^i}((\sigma_{ij} - \sigma_{0,ij})^4 \mid \mathbb{X}_n)\}^{1/2} E_{\Sigma_0} \{P^{\pi^i}(|\sigma_{ij} - \sigma_{0,ij}| \geq \frac{\gamma}{2} \left(\frac{\log p}{n}\right)^{1/2} \mid \mathbb{X}_n)\}^{1/2},$$

and

$$E_{\Sigma_0} \{E^{\pi^i}((\sigma_{ij} - \sigma_{0,ij})^4 \mid \mathbb{X}_n)\} \leq E_{\Sigma_0} \{E^{\pi^i}(\|\Sigma_{\{i,j\} \times \{i,j\}} - (\Sigma_0)_{\{i,j\} \times \{i,j\}}\|_2^4 \mid \mathbb{X}_n)\}.$$

Since  $[\Sigma_{\{i,j\} \times \{i,j\}} \mid \mathbb{X}_n] \sim IW_2(n + \nu_n - 2p + 4, A_{\{i,j\} \times \{i,j\}} + nS_{\{i,j\} \times \{i,j\}})$  (Press; 2012, Theorem 5.2.3), Lemma 6.1 in the supplementary material of Lee et al. (2021) gives that there exist a positive constant  $C_1$  such that

$$E_{\Sigma_0} \{E^{\pi^i}(\|\Sigma_{\{i,j\} \times \{i,j\}} - (\Sigma_0)_{\{i,j\} \times \{i,j\}}\|_2^4 \mid \mathbb{X}_n)\}^{1/2} \leq \frac{C_1}{n}, \quad (S5)$$

for all sufficiently large  $n$ . Lemma S1.2 gives that there exist some positive constants  $C_2$  and  $\lambda_1$  such that

$$E_{\Sigma_0} \{P^{\pi^i}(|\sigma_{ij} - \sigma_{0,ij}| \geq \frac{\gamma}{2} \left(\frac{\log p}{n}\right)^{1/2} \mid \mathbb{X}_n)\}^{1/2} \leq C_2 \{\exp(-\lambda_1 n) + \exp(-\lambda_1 \gamma^2 \log p / 2)\},$$

for all sufficiently large  $n$ . Thus, we get

$$(S3) \leq C_3 \frac{1}{n} \left( \frac{1}{p^{\lambda_1 \gamma^2 / 2 - 3}} + p^3 \exp(-\lambda_1 n / 2) \right),$$

for a positive constant  $C_3$ . If  $\gamma$  is a sufficiently large constant and  $\log p = o(n)$ , then  $(S3) = O(1/n)$ .

For the upper bound of (S4), there exist positive constants  $C_4$  and  $\lambda_2$  such that

$$\begin{aligned} (S4) &\leq \sum_{ij} \sigma_{0,ij}^2 I(|\sigma_{0,ij}| \geq 4\gamma(\log p/n)^{1/2}) E_{\Sigma_0} \{P^{\pi^i}(|\sigma_{ij} - \sigma_{0,ij}| > \frac{3}{4}|\sigma_{0,ij}| \mid \mathbb{X}_n)\} \\ &\leq \sum_{ij} \sigma_{0,ij}^2 I(|\sigma_{0,ij}| \geq 4\gamma(\log p/n)^{1/2}) E_{\Sigma_0} \{P^{\pi^i}(\|\Sigma_{\{i,j\} \times \{i,j\}} - (\Sigma_0)_{\{i,j\} \times \{i,j\}}\|_2 > \frac{3}{4}|\sigma_{0,ij}| \mid \mathbb{X}_n)\} \\ &\leq C_4 \frac{p^2}{n} \sup_{ij} \{n\sigma_{0,ij}^2 \exp(-n\lambda_2\sigma_{0,ij}^2) I(n\sigma_{0,ij}^2 \geq 16\gamma^2 \log p)\} \\ &\leq C_4 \frac{p^2}{n} 16\gamma^2 \log p \exp(-\lambda_2 16\gamma^2 \log p) \\ &\leq \frac{C_4}{n} \exp(-\lambda_2 16\gamma^2 \log p + 2 \log p + \log \log p), \end{aligned} \quad (S6)$$

for all sufficiently large  $n$ . The third inequality holds by Lemma 6.2 in the supplementary material of Lee et al. (2021). If  $\gamma$  is a sufficiently large constant and  $\log p = o(n)$ , then  $(S4) = O(1/n)$ .  $\square$

*Proof of Theorem 2.1.* By Lemma 2.1 in the supplementary material of Lee et al. (2021), we have

$$\|H_{\gamma}^{(\epsilon_n)}(\Sigma) - \Sigma_0\|_2^2 \leq 2^3 \|H_{\gamma}(\Sigma) - \Sigma_0\|_2^2 + 4\epsilon_n^2.$$

Lemma S1.1 gives that there exist a positive constant  $C_1$  such that

$$\begin{aligned} \|H_\gamma(\Sigma) - \Sigma_0\|_2^2 &\leq \|H_\gamma(\Sigma) - \Sigma_0\|_1^2 \\ &\leq C_1(c_{n,p}^2 \left(\frac{\log p}{n}\right)^{1-q} + \frac{\log p}{n}) + 2\|D\|_1^2, \end{aligned}$$

where  $D = (d_{ij})_{1 \leq i, j \leq p}$ ,  $d_{ij} = (H_\gamma(\Sigma)_{ij} - \sigma_{0,ij})I(A_{ij}^c)$ , and

$$A_{ij} = \left\{ |(H_\gamma(\Sigma))_{ij} - \sigma_{0,ij}| \leq 4 \min \left\{ |\sigma_{0,ij}|, \gamma \sqrt{\frac{\log p}{n}} \right\} \right\}.$$

By applying Lemma S1.3 to the term  $\|D_1\|^2$ , we complete the proof. □

## S2 Proof of Theorem 3.1

In this section, we prove Theorem 3.1 to show the upper bound of the post-processed posterior in the respect of the global minimum variance portfolio. Before proving the theorem, we present two lemmas and two corollaries from one of the lemma.

**Lemma S2.1.** *Let  $M$  be an arbitrary positive constant. If  $(\nu_n - 2p) \vee \|A\| = o(n)$  and  $x$  satisfies*

$$\left[ x - \left\{ C_1 c_{n,p} \left( \frac{\log p}{n} \right)^{(1-q)/2} + 4\gamma \left( \frac{\log p}{n} \right)^{1/2} \right\} \right] > M,$$

*for a positive constant  $C_1$ , then there exist positive constants  $C, \lambda$  such that*

$$P(\|H_\gamma(\Sigma) - \Sigma_0\|_1 > x) \leq C(2p^2 \exp(-\lambda n) + p^2 \exp(-\lambda n^\delta) + n^{(2-\lambda\gamma)(1-\delta)/2}),$$

*for all  $\gamma > 2/\lambda$ , all sufficiently large  $n$  and all  $\delta \in (0, 1)$ .*

*Proof.* Using Lemma S1.1, we have

$$\begin{aligned} P^{\pi^i}(\|H_\gamma(\Sigma) - \Sigma_0\|_1 > x \mid \mathbb{X}_n) &\leq P^{\pi^i}(\|D\|_1 > x - s_n \mid \mathbb{X}_n) \\ &\leq p \sup_j P^{\pi^i} \left( \sum_{i=1}^p |d_{ij}| > x - s_n \mid \mathbb{X}_n \right) \\ &\leq p^2 \sup_{i,j} P^{\pi^i}(|d_{ij}| > (x - s_n)/p \mid \mathbb{X}_n), \end{aligned}$$

where  $s_n = C_1 c_{n,p} ((\log p)/n)^{(1-q)/2} + 4\gamma ((\log p)/n)^{1/2}$  for a positive constant  $C_1$ . We show the upper bound of  $\sup_{i,j} P^{\pi^i}(|d_{ij}| > (x - s_n)/p \mid \mathbb{X}_n)$  for the two cases:  $p \leq n^{(1-\delta)/2}$  and  $p > n^{(1-\delta)/2}$ , where  $\delta$  is an

arbitrary real number in  $(0, 1)$ . First, we consider the case  $p \leq n^{(1-\delta)/2}$ . We have

$$\begin{aligned}
& P^{\pi^i}(|d_{ij}| > (x - s_n)/p \mid \mathbb{X}_n) \\
& \leq P^{\pi^i}(|H_\gamma(\Sigma)_{ij} - \sigma_{0,ij}| > (x - s_n)/p \mid \mathbb{X}_n) \\
& \leq P^{\pi^i}(|\sigma_{ij} - \sigma_{0,ij}| > (x - s_n)/p \mid \mathbb{X}_n) + E^{\pi^i}(I(|\sigma_{0,ij}| > (x - s_n)/p)I(|\sigma_{ij}| < \gamma((\log p)/n)^{1/2}) \mid \mathbb{X}_n) \\
& \leq P^{\pi^i}(|\sigma_{ij} - \sigma_{0,ij}| > (x - s_n)/p \mid \mathbb{X}_n) + P^{\pi^i}(|\sigma_{0,ij}| - |\sigma_{ij}| > (x - s_n)/p - \gamma((\log p)/n)^{1/2} \mid \mathbb{X}_n) \\
& \leq 2P^{\pi^i}(|\sigma_{ij} - \sigma_{0,ij}| > (x - s_n)/p - \gamma(\log p/n)^{1/2} \mid \mathbb{X}_n) \\
& \leq 2P^{\pi^i}(|\sigma_{ij} - \sigma_{0,ij}| > (x - s_n)n^{(\delta-1)/2} - \gamma((1-\delta)(\log n)/(2n))^{1/2} \mid \mathbb{X}_n),
\end{aligned}$$

where the assumption  $p \leq n^{(1-\delta)}$  is used only in the last inequality. For all sufficiently large  $n$ , we have

$$(x - s_n)n^{(\delta-1)/2} - \gamma((1-\delta)(\log n)/(2n))^{1/2} > Mn^{(\delta-1)/2}/2.$$

Thus, there exist some positive constants  $C_2$  and  $\lambda_1$  such that

$$P^{\pi^i}(|d_{ij}| > (x - s_n)/p \mid \mathbb{X}_n) \leq C_2[\exp(-n\lambda_1) + \exp(-\lambda_1 n^\delta)], \quad (\text{S7})$$

for all sufficiently large  $n$  by Lemma S1.2.

Next we consider the second case  $p > n^{(1-\delta)/2}$ . Since  $x - s_n > 0$ , we have

$$P^{\pi^i}(|d_{ij}| > (x - s_n)/p \mid \mathbb{X}_n) \leq P^{\pi^i}(A_{ij}^c \mid \mathbb{X}_n).$$

Note that

$$\begin{aligned}
I(A_{ij}^c) &= I(A_{ij}^c)\{I(|\sigma_{ij}| \geq \gamma(\log p/n)^{1/2}) + I(|\sigma_{ij}| < \gamma(\log p/n)^{1/2})\} \\
&\leq I(|\sigma_{ij} - \sigma_{0,ij}| \geq \frac{\gamma}{2}\left(\frac{\log p}{n}\right)^{1/2}) + I(|\sigma_{ij} - \sigma_{0,ij}| \geq 3\gamma\left(\frac{\log p}{n}\right)^{1/2}),
\end{aligned}$$

by (S1) and (S2). Thus, by Lemma S1.2, there exist some positive constants  $C_3$  and  $\lambda_2$  such that

$$P^{\pi^i}(A_{ij}^c \mid \mathbb{X}_n) \leq C_3(\exp(-\lambda_2 n) + \exp(-\lambda_2 \gamma \log p)). \quad (\text{S8})$$

If  $\gamma$  is a sufficiently large positive constant such that  $\gamma > 2/\lambda_2$ , then

$$\begin{aligned}
p^2 \sup_{i,j} P^{\pi^i}(A_{ij}^c \mid \mathbb{X}_n) &\leq C_3(p^2 \exp(-\lambda_2 n) + p^{2-\lambda_2 \gamma}) \\
&\leq C_3(p^2 \exp(-\lambda_2 n) + n^{(2-\lambda_2 \gamma)(1-\delta)/2}).
\end{aligned} \quad (\text{S9})$$

The assumption  $p > n^{(1-\delta)/2}$  is used only in the last inequality. By combining (S7) and (S9), the proof is completed.  $\square$

Using Lemma S2.1, we derive two Corollaries S2.2 and S2.3.

**Corollary S2.2.** Suppose the same setting of Lemma S2.1. If

$$x > 2\|\Sigma_0\| + \left\{ C_1 c_{n,p} \left( \frac{\log p}{n} \right)^{(1-q)/2} + 4\gamma \left( \frac{\log p}{n} \right)^{1/2} \right\}$$

for a positive constant  $C_1$ , then there exist positive constants  $C, \lambda$  such that

$$P^{\pi^i}(\lambda_{\max}(H_\gamma(\Sigma)) > x) \leq C(2p^2 \exp(-\lambda n) + p^2 \exp(-\lambda n^\delta) + n^{(2-\lambda\gamma)(1-\delta)/2}),$$

for all  $\gamma > 2/\lambda$ , all sufficiently large  $n$  and all  $\delta \in (0, 1)$ .

*Proof.* We have

$$\begin{aligned} P^{\pi^i}(\lambda_{\max}(H_\gamma(\Sigma)) > x \mid \mathbb{X}_n) &\leq P^{\pi^i}(\|H_\gamma(\Sigma) - \Sigma_0\| > x - \|\Sigma_0\| \mid \mathbb{X}_n) \\ &\leq P^{\pi^i}(\|H_\gamma(\Sigma) - \Sigma_0\|_1 > x - \|\Sigma_0\| \mid \mathbb{X}_n) \end{aligned}$$

Since  $x - \|\Sigma_0\| > \|\Sigma_0\| + \left\{ C_1 c_{n,p} \left( \frac{\log p}{n} \right)^{(1-q)/2} + 4\gamma \left( \frac{\log p}{n} \right)^{1/2} \right\}$ , we apply Lemma S2.1 and the proof is completed.  $\square$

**Corollary S2.3.** Suppose the same setting of Lemma S2.1. If

$$x < \lambda_{\min}(\Sigma_0)/2 - \left\{ C_1 c_{n,p} \left( \frac{\log p}{n} \right)^{(1-q)/2} + 4\gamma \left( \frac{\log p}{n} \right)^{1/2} \right\},$$

for a positive constant  $C_1$ , then there exist positive constants  $C, \lambda$  such that

$$P^{\pi^i}(\lambda_{\min}(H_\gamma(\Sigma)) < x \mid \mathbb{X}_n) \leq C(2p^2 \exp(-\lambda n) + p^2 \exp(-\lambda n^\delta) + n^{(2-\lambda\gamma)(1-\delta)/2}),$$

for all  $\gamma > 2/\lambda$ , all sufficiently large  $n$  and all  $\delta \in (0, 1)$ .

*Proof.* We have

$$\begin{aligned} P^{\pi^i}(\lambda_{\min}(H_\gamma(\Sigma)) < x \mid \mathbb{X}_n) &\leq P^{\pi^i}(\lambda_{\min}(\Sigma_0) - \|H_\gamma(\Sigma) - \Sigma_0\| < x \mid \mathbb{X}_n) \\ &\leq P^{\pi^i}(\|H_\gamma(\Sigma) - \Sigma_0\|_1 > \lambda_{\min}(\Sigma_0) - x \mid \mathbb{X}_n) \end{aligned}$$

Since  $\lambda_{\min}(\Sigma_0) - x > \lambda_{\min}(\Sigma_0)/2 + \left\{ C_1 c_{n,p} \left( \frac{\log p}{n} \right)^{(1-q)/2} + 4\gamma \left( \frac{\log p}{n} \right)^{1/2} \right\}$ , the proof is completed by Lemma S2.1.  $\square$

**Lemma S2.4.** If  $c_{n,p}^4 (\log p/n)^{2(1-q)} + \gamma^4 ((\log p)/n)^2$  is bounded and  $(\nu_n - 2p) \vee \|A\| = o(n)$ , then  $E_{\Sigma_0} E^{\pi^i}(\|(\Sigma_0 - H_\gamma^{(\epsilon_n)}(\Sigma))\Sigma_0^{-1}\mathbf{1}\|^4 \mid \mathbb{X}_n)$  is bounded by a positive constant for all sufficiently large  $p$ .

*Proof.* By Lemma S1.1, it suffices to show that  $E_{\Sigma_0}\{E^{\pi^i}(\|D\|_1^4 \mid \mathbb{X}_n)\}$  is bounded. We have

$$\begin{aligned}
E_{\Sigma_0}\{E^{\pi^i}(\|D\|_2^4 \mid \mathbb{X}_n)\} &\leq E_{\Sigma_0}\{E^{\pi^i}(\sup_i (\sum_j |d_{ij}|)^4 \mid \mathbb{X}_n)\} \\
&\leq p^3 \sum_{i,j} E_{\Sigma_0}\{E^{\pi^i}(|d_{ij}|^4 \mid \mathbb{X}_n)\} \\
&\leq p^5 \sup_{i,j} E_{\Sigma_0}\{E^{\pi^i}(|H_\gamma(\Sigma)_{ij} - \sigma_{0,ij}|^4 I(A_{ij}^c) \mid \mathbb{X}_n)\} \\
&\leq p^5 \sup_{i,j} E_{\Sigma_0}\{E^{\pi^i}(|\sigma_{ij} - \sigma_{0,ij}|^4 I(A_{ij}^c) \mid \mathbb{X}_n)\} \\
&\quad + p^5 \sup_{i,j} E_{\Sigma_0}\{E^{\pi^i}(|\sigma_{0,ij}|^4 I(A_{ij}^c) I(|\sigma_{ij} - \sigma_{0,ij}| < \gamma(\log p/n)^{1/2}) \mid \mathbb{X}_n)\}
\end{aligned}$$

By (S8) and Lemma 6.1 in the supplementary material of Lee et al. (2021), there exist positive constants  $C_1$  and  $\lambda_1$  such that

$$\begin{aligned}
E_{\Sigma_0}\{E^{\pi^i}(|\sigma_{ij} - \sigma_{0,ij}|^4 I(A_{ij}^c) \mid \mathbb{X}_n)\} &\leq [E\{(\sigma_{ij} - \sigma_{0,ij})^8 \mid \mathbb{X}_n\}]^{1/2} P(A_{ij}^c \mid \mathbb{X}_n)^{1/2} \\
&\leq \{E(\|\Sigma_{\{i,j\} \times \{i,j\}} - (\Sigma_0)_{\{i,j\} \times \{i,j\}}\|_2^8 \mid \mathbb{X}_n)\}^{1/2} P(A_{ij} \mid \mathbb{X}_n)^{1/2} \\
&\leq C_1 \frac{p^2}{n^2} p^{-\lambda_1 \gamma}.
\end{aligned}$$

Next, we have

$$\begin{aligned}
&E_{\Sigma_0}\{E^{\pi^i}(|\sigma_{0,ij}|^4 I(A_{ij}^c) I(|\sigma_{ij} - \sigma_{0,ij}| < \gamma(\log p/n)^{1/2}) \mid \mathbb{X}_n)\} \\
&\leq E_{\Sigma_0}\{E^{\pi^i}(|\sigma_{0,ij}|^4 I(|\sigma_{ij} - \sigma_{0,ij}| \geq 3|\sigma_{0,ij}|/4) I(|\sigma_{0,ij}| > 4\gamma\sqrt{\frac{\log p}{n}}) \mid \mathbb{X}_n)\} \\
&\leq |\sigma_{0,ij}|^4 I(|\sigma_{0,ij}| > 4\gamma\sqrt{\frac{\log p}{n}}) E_{\Sigma_0}\{P^{\pi^i}(\|\Sigma_{\{i,j\} \times \{i,j\}} - (\Sigma_0)_{\{i,j\} \times \{i,j\}} > 3|\sigma_{0,ij}|/4 \mid \mathbb{X}_n)\} \\
&\leq |\sigma_{0,ij}|^4 I(|\sigma_{0,ij}| > 4\gamma\sqrt{\frac{\log p}{n}}) \exp(-n\lambda_1\sigma_{0,ij}^2) \\
&= \frac{1}{n^2} (n\sigma_{0,ij}^2)^2 \exp(-n\lambda_1\sigma_{0,ij}^2) I(n\sigma_{0,ij}^2 > 16\gamma^2 \log p),
\end{aligned}$$

where the first inequality is satisfied by (S2). Note that  $f(x) = x^2 \exp(-\lambda_1 x)$  is a decreasing function when  $x > 2/\lambda_1$ . If  $p$  is large enough to satisfy  $16\gamma^2 \log p > 2/\lambda_1$ , then

$$\begin{aligned}
&\frac{1}{n^2} (n\sigma_{0,ij}^2)^2 \exp(-n\lambda_1\sigma_{0,ij}^2) I(n\sigma_{0,ij}^2 > 16\gamma^2 \log p) \\
&\leq \frac{1}{n^2} (16\gamma^2 \log p)^2 \exp(-\lambda_1 16\gamma^2 \log p) \\
&= \frac{(16\gamma^2 \log p)^2}{n^2 p^{\lambda_1 16\gamma^2}}.
\end{aligned}$$

Thus,

$$E_{\Sigma_0}\{E^{\pi^i}(\|D\|_2^4 \mid \mathbb{X}_n)\} \leq \frac{p^{5-\lambda_1 \gamma}}{n^2} + \frac{(16\gamma^2 \log p)^2}{n^2 p^{\lambda_1 16\gamma^2}},$$

which is bounded by a positive constant when  $\gamma$  is a sufficiently large constant.  $\square$

Using the lemmas and corollaries, we prove Theorem 3.1.

*Proof of Theorem 3.1.* We have

$$\begin{aligned}
\left\| \frac{H_\gamma^{(\epsilon_n)}(\Sigma)^{-1} \mathbf{1}}{\mathbf{1}^T H_\gamma^{(\epsilon_n)}(\Sigma)^{-1} \mathbf{1}} - \frac{\Sigma_0^{-1} \mathbf{1}}{\mathbf{1}^T \Sigma_0^{-1} \mathbf{1}} \right\|_2^2 &\leq \frac{2}{|\mathbf{1}^T H_\gamma^{(\epsilon_n)}(\Sigma)^{-1} \mathbf{1}|^2} \|(H_\gamma^{(\epsilon_n)}(\Sigma)^{-1} - \Sigma_0^{-1}) \mathbf{1}\|_2^2 \\
&\quad + \frac{2\|\Sigma_0^{-1} \mathbf{1}/\sqrt{p}\|^2}{|(\mathbf{1}/\sqrt{p})^T \Sigma_0^{-1} \mathbf{1}/\sqrt{p}|^2} \frac{|(\mathbf{1}/\sqrt{p})^T (H_\gamma^{(\epsilon_n)}(\Sigma)^{-1} - \Sigma_0^{-1}) \mathbf{1}|^2}{|\mathbf{1}^T H_\gamma^{(\epsilon_n)}(\Sigma)^{-1} \mathbf{1}|^2} \\
&\leq \frac{2\|(H_\gamma^{(\epsilon_n)}(\Sigma)^{-1} - \Sigma_0^{-1}) \mathbf{1}\|_2^2}{|\mathbf{1}^T H_\gamma^{(\epsilon_n)}(\Sigma)^{-1} \mathbf{1}|^2} \left(1 + \frac{\|\Sigma_0^{-1}\|^2}{\lambda_{\min}(\Sigma_0^{-1})^2}\right) \\
&\leq \frac{2}{p^2} \|(H_\gamma^{(\epsilon_n)}(\Sigma)^{-1} - \Sigma_0^{-1}) \mathbf{1}\|_2^2 \lambda_{\max}(H_\gamma^{(\epsilon_n)}(\Sigma))^2 \left(1 + \frac{\|\Sigma_0^{-1}\|^2}{\lambda_{\min}(\Sigma_0^{-1})^2}\right) \\
&\leq \frac{2}{p^2} \|(\Sigma_0 - H_\gamma^{(\epsilon_n)}(\Sigma)) \Sigma_0^{-1} \mathbf{1}\|_2^2 \|H_\gamma^{(\epsilon_n)}(\Sigma)^{-1}\|^2 \|H_\gamma^{(\epsilon_n)}(\Sigma)\|^2 \left(1 + \frac{\|\Sigma_0^{-1}\|^2}{\lambda_{\min}(\Sigma_0^{-1})^2}\right).
\end{aligned}$$

Next, for an arbitrary positive constant  $C_1$ , we have

$$\begin{aligned}
&E^{\pi^i}(\|(\Sigma_0 - H_\gamma^{(\epsilon_n)}(\Sigma)) \Sigma_0^{-1} \mathbf{1}\|_2^2 \|H_\gamma^{(\epsilon_n)}(\Sigma)^{-1}\|^2 \|H_\gamma^{(\epsilon_n)}(\Sigma)\|^2 \mid \mathbb{X}_n) \\
&\leq C_1^4 E^{\pi^i}(\|(\Sigma_0 - H_\gamma^{(\epsilon_n)}(\Sigma)) \Sigma_0^{-1} \mathbf{1}\|_2^2 \mid \mathbb{X}_n) \tag{S10} \\
&\quad + E^{\pi^i}(\|(\Sigma_0 - H_\gamma^{(\epsilon_n)}(\Sigma)) \Sigma_0^{-1} \mathbf{1}\|^4 \mid \mathbb{X}_n)^{1/2} E^{\pi^i}\{I(\|H_\gamma^{(\epsilon_n)}(\Sigma)^{-1}\| > C_1) I(\|H_\gamma^{(\epsilon_n)}(\Sigma)\| > C_1) \mid \mathbb{X}_n\} \tag{S11}
\end{aligned}$$

We show the upper bound of (S11). Lemma S2.4 shows that  $E^{\pi^i}(\|(\Sigma_0 - H_\gamma^{(\epsilon_n)}(\Sigma)) \Sigma_0^{-1} \mathbf{1}\|^4 \mid \mathbb{X}_n)^{1/2}$  is bounded by a positive constant. There exist positive constants  $C_2$  and  $\lambda_1$  such that

$$\begin{aligned}
&E^{\pi^i}\{I(\|H_\gamma^{(\epsilon_n)}(\Sigma)^{-1}\| > C_1) I(\|H_\gamma^{(\epsilon_n)}(\Sigma)\| > C_1) \mid \mathbb{X}_n\} \\
&\leq E^{\pi^i}\{I(\|H_\gamma(\Sigma)^{-1}\| > C_1) I(\|H_\gamma(\Sigma)\| > C_1) \mid \mathbb{X}_n\} \\
&\quad + E^{\pi^i}\{I(\lambda_{\min}(H_\gamma(\Sigma)) < \epsilon_n) \mid \mathbb{X}_n\} \\
&\leq P^{\pi^i}(\|H_\gamma(\Sigma)\| > C_1 \mid \mathbb{X}_n)^{1/2} P^{\pi^i}(\lambda_{\min}(H_\gamma(\Sigma)) < C_1^{-1} \mid \mathbb{X}_n)^{1/2} \\
&\quad + E^{\pi^i}\{I(\lambda_{\min}(H_\gamma(\Sigma)) < \epsilon_n) \mid \mathbb{X}_n\} \\
&\leq P^{\pi^i}(\|H_\gamma(\Sigma)\| > C_1 \mid \mathbb{X}_n)^{1/2} P^{\pi^i}(\lambda_{\min}(H_\gamma(\Sigma)) < C_1^{-1} \mid \mathbb{X}_n)^{1/2} \\
&\quad + P^{\pi^i}(\lambda_{\min}(\Sigma_0) - \epsilon_n < \|H_\gamma(\Sigma) - \Sigma_0\| \mid \mathbb{X}_n) \\
&\leq C_2(p^2 \exp(-\lambda_1 n) + p^2 \exp(-\lambda_1 n^\delta) + n^{(2-\lambda_1 \gamma)(1-\delta)/2}),
\end{aligned}$$

for all sufficiently large  $n$ . The last inequality is satisfied by Corollaries S2.2, S2.3 and Lemma S2.1 since  $\epsilon_n < \lambda_{\min}(\Sigma_0)/2$  and  $c_{n,p}((\log p)/n)^{(1-q)/2} + 4\gamma((\log p)/n)^{1/2} \longrightarrow 0$  as  $n \longrightarrow \infty$ .

We show the upper bound of (S10). There exists positive constant  $C_3$  and  $\lambda_2$  such that

$$\begin{aligned}
& E_{\Sigma_0} E^{\pi^i} (\|(\Sigma_0 - H_{\gamma}^{(\epsilon_n)}(\Sigma)) \Sigma_0^{-1} \mathbf{1}\|^2 \mid \mathbb{X}_n) \\
\leq & E_{\Sigma_0} E^{\pi^i} (\|(\Sigma_0 - H_{\gamma}(\Sigma)) \Sigma_0^{-1} \mathbf{1}\|^2 \mid \mathbb{X}_n) \\
& + E_{\Sigma_0} E^{\pi^i} (\|(\Sigma_0 - H_{\gamma}^{(\epsilon_n)}(\Sigma))\|^2 I(\lambda_{\min}(H_{\gamma}(\Sigma)) < \epsilon_n) \mid \mathbb{X}_n) \|\Sigma_0^{-1} \mathbf{1}\|^2 \\
\leq & 2E_{\Sigma_0} E^{\pi^i} (\|diag(\Sigma_0 - H_{\gamma}(\Sigma)) \Sigma_0^{-1} \mathbf{1}\|^2 + 2\|diag^c(\Sigma_0 - H_{\gamma}(\Sigma)) \Sigma_0^{-1} \mathbf{1}\|^2 \mid \mathbb{X}_n) \\
& + \|\Sigma_0^{-1} \mathbf{1}\|^2 E_{\Sigma_0} E^{\pi^i} (\|(\Sigma_0 - H_{\gamma}^{(\epsilon_n)}(\Sigma))\|^4 \mid \mathbb{X}_n)^{1/2} E_{\Sigma_0} P^{\pi^i} (\lambda_{\min}(\Sigma_0) - \epsilon_n < \|H_{\gamma}(\Sigma) - \Sigma_0\| \mid \mathbb{X}_n)^{1/2} \\
\leq & 2E_{\Sigma_0} E^{\pi^i} (\|diag(\Sigma_0 - H_{\gamma}(\Sigma)) \Sigma_0^{-1} \mathbf{1}\|^2 + 2\|diag^c(\Sigma_0 - H_{\gamma}(\Sigma)) \Sigma_0^{-1} \mathbf{1}\|^2 \mid \mathbb{X}_n) \\
& + C_3 p(p^2 \exp(-\lambda_2 n) + p^2 \exp(-\lambda_2 n^\delta) + n^{(2-\lambda_2 \gamma)(1-\delta)/2}),
\end{aligned}$$

for all sufficiently large  $n$ . The last inequality is satisfied by Lemma S2.1. Next, we have

$$\begin{aligned}
& E_{\Sigma_0} E^{\pi^i} (\|diag(\Sigma_0 - H_{\gamma}(\Sigma)) \Sigma_0^{-1} \mathbf{1}\|^2 \mid \mathbb{X}_n) \\
\leq & \|\Sigma_0^{-1} \mathbf{1}\|^2 \sum_{i=1}^p E_{\Sigma_0} E^{\pi^i} ((\Sigma_{0,ii} - H_{\gamma}(\Sigma)_{ii})^2 \mid \mathbb{X}_n) \\
\leq & 2\|\Sigma_0^{-1} \mathbf{1}\|^2 \sum_{i=1}^{p-1} E_{\Sigma_0} E^{\pi^i} (\|(\Sigma_0)_{i:i+1, i:i+1} - H_{\gamma}(\Sigma)_{i:i+1, i:i+1}\|^2 \mid \mathbb{X}_n)
\end{aligned}$$

We apply Theorem 2.1 considering that the true covariance is  $(\Sigma_0)_{i:i+1, i:i+1}$ . There exists a positive constant  $C_4$  such that

$$\sum_{i=1}^{p-1} E_{\Sigma_0} E^{\pi^i} (\|(\Sigma_0)_{i:i+1, i:i+1} - H_{\gamma}(\Sigma)_{i:i+1, i:i+1}\|^2 \mid \mathbb{X}_n) \leq C_4 \frac{p}{n},$$

for all sufficiently large  $n$ . Lemmas S1.1 and S1.3 give that there exist a positive constant  $C_4$  such that

$$\begin{aligned}
& E_{\Sigma_0} E^{\pi^i} (\|diag^c(\Sigma_0 - H_{\gamma}(\Sigma)) \Sigma_0^{-1} \mathbf{1}\|^2 \mid \mathbb{X}_n) \\
\leq & \|\Sigma_0^{-1} \mathbf{1}\|^2 E_{\Sigma_0} E^{\pi^i} \left( 2\|D\|_1^2 + 2\left\{ 4C c_{n,p} \left( \frac{\log p}{n} \right)^{(1-q)/2} \right\}^2 \mid \mathbb{X}_n \right) \\
\leq & p C_4 \left( \frac{1}{n} + c_{n,p}^2 \left( \frac{\log p}{n} \right)^{(1-q)} \right),
\end{aligned}$$

for all sufficiently large  $n$ .

Collecting all the inequalities above, we have

$$\begin{aligned}
& E_{\Sigma_0} E^{\pi^i} (\|(\Sigma_0 - H_{\gamma}^{(\epsilon_n)}(\Sigma)) \Sigma_0^{-1} \mathbf{1}\|^2 \mid \mathbb{X}_n) \\
\leq & \frac{1}{p} (p^2 \exp(-\lambda_2 n) + p^2 \exp(-\lambda_2 n^\delta) + n^{(2-\lambda_2 \gamma)(1-\delta)/2} + \frac{1}{n} + c_{n,p}^2 \left( \frac{\log p}{n} \right)^{(1-q)}),
\end{aligned}$$

and

$$E_{\Sigma_0} E^{\pi^i} \left( \left\| \frac{H_{\gamma}^{(\epsilon_n)}(\Sigma)^{-1} \mathbf{1}}{\mathbf{1}^T H_{\gamma}^{(\epsilon_n)}(\Sigma)^{-1} \mathbf{1}} - \frac{\Sigma_0^{-1} \mathbf{1}}{\mathbf{1}^T \Sigma_0^{-1} \mathbf{1}} \right\|_2^2 \mid \mathbb{X}_n \right) \lesssim \frac{1}{p} \left( \frac{1}{n} + c_{n,p}^2 \left( \frac{\log p}{n} \right)^{(1-q)} \right).$$

Since

$$\left\| \frac{\Sigma_0^{-1} \mathbf{1}}{\mathbf{1}^T \Sigma_0^{-1} \mathbf{1}} \right\|^2 \leq \frac{\|\Sigma_0^{-1}\|^2 \|\Sigma_0\|^2}{p},$$

the proof is completed. □

### S3 Proof of Lemmas 3.2 and 3.3

For the proof of Lemma 3.2, we present Lemma S3.1.

**Lemma S3.1.** *Suppose the notation of  $\mathcal{G}^{(1)}$  in 1. If  $\tau/\sqrt{n} \leq M/3$  and  $\tau/M \leq 1/3$ , then there exists a positive constant  $C$  such that*

$$\min_{\{(\theta, \theta') \in \{0,1\}^{p'} : H(\theta, \theta')=1\}} \|\mathbb{P}_\theta \wedge \mathbb{P}_{\theta'}\| \geq C.$$

*Proof.* Since  $\|\mathbb{P}_\theta \wedge \mathbb{P}_{\theta'}\| = 1 - 0.5\|\mathbb{P}_\theta - \mathbb{P}_{\theta'}\|_1$ , it suffices to show  $\|\mathbb{P}_\theta - \mathbb{P}_{\theta'}\|_1 \leq 1$ . We have

$$\begin{aligned} \|\mathbb{P}_\theta - \mathbb{P}_{\theta'}\|_1^2 &\leq 2K(\mathbb{P}_{\theta'} | \mathbb{P}_\theta) \\ &\leq n[\text{tr}(\Sigma(\theta')\Sigma^{-1}(\theta)) - \log \det(\Sigma(\theta')\Sigma^{-1}(\theta)) - p]. \end{aligned}$$

Let  $D := \Sigma^{-1}(\theta) - \Sigma^{-1}(\theta')$  and  $j$  be the index such that  $D_{jj} > 0$ . Note that there is only one index of which  $D_{jj}$  is positive when  $H(\theta, \theta') = 1$ . Let  $x = \Sigma(\theta')_{jj} D_{jj}$ . We have

$$\begin{aligned} \text{tr}(\Sigma(\theta')\Sigma^{-1}(\theta)) - p &= \text{tr}(\Sigma(\theta')D) \\ &= x \\ \log \det(\Sigma(\theta')\Sigma^{-1}(\theta)) &= \log \det(\Sigma(\theta')D + I_p) \\ &= \log(1 + x), \end{aligned}$$

thus

$$\begin{aligned} \|\mathbb{P}_\theta - \mathbb{P}_{\theta'}\|_1^2 &\leq n(x - \log(1 + x)) \\ &= \frac{n}{(1 + \xi)^2} \frac{x^2}{2}, \end{aligned}$$

where  $\xi \in [-|x|, |x|]$ . Since  $|x| \leq (\tau/\sqrt{n})/(M - \tau/\sqrt{n})$  and  $\tau/\sqrt{n} \leq M/3$ ,

$$\begin{aligned} \|\mathbb{P}_\theta - \mathbb{P}_{\theta'}\|_1^2 &\leq \frac{nx^2}{2(1 + \xi)^2} \\ &\leq \frac{nx^2}{2(1 - 0.5)^2} \\ &\leq \frac{9\tau^2}{2M^2}. \end{aligned}$$

Since  $\tau/M \leq 1/3$ , the proof is completed.  $\square$

*Proof of Lemma 3.2.* By the definition of  $\Sigma(\theta)^{-1}$ ,

$$\frac{\Sigma(\theta)^{-1}\mathbf{1}}{\mathbf{1}^T \Sigma^{-1}(\theta)\mathbf{1}} = \frac{1}{p} \frac{((\Sigma(\theta)^{-1})_{11}, \dots, (\Sigma(\theta)^{-1})_{pp})^T}{M + |\theta|\tau/(p\sqrt{n})},$$

and

$$\frac{\Sigma(\theta)^{-1}\mathbf{1}}{\mathbf{1}^T \Sigma^{-1}(\theta)\mathbf{1}} - \frac{\Sigma(\theta')^{-1}\mathbf{1}}{\mathbf{1}^T \Sigma^{-1}(\theta')\mathbf{1}} = \frac{(v_1, v_2, \dots, v_p)^T}{p(M + |\theta|\tau/(p\sqrt{n}))(M + |\theta'|\tau/(p\sqrt{n}))},$$

for some  $v_1, v_2, \dots, v_p \in \mathbb{R}$ . When  $i \leq p'$  and  $\theta_i \neq \theta'_i$ ,

$$v_i = M\tau \frac{|\theta'| - |\theta|}{p\sqrt{n}} + |\theta_i - \theta'_i| \frac{\tau}{\sqrt{n}} \left( M + \tau \frac{|\theta'|\theta_i + |\theta|\theta'_i}{p\sqrt{n}} \right),$$

and

$$\begin{aligned} |v_i| &\geq \frac{\tau}{\sqrt{n}} \left( M + \tau \frac{|\theta'|\theta_i + |\theta|\theta'_i}{p\sqrt{n}} \right) - M\tau/(2\sqrt{n}) \\ &\geq M\tau/(2\sqrt{n}), \end{aligned}$$

since  $||\theta'| - |\theta|| < p/2$ . Thus, we have

$$\begin{aligned} ||(v_1, \dots, v_p)^T||_2^2 &\geq H(\theta, \theta') M^2 \tau^2 / (4n), \\ \min_{H(\theta, \theta') \geq 1} \frac{||w_{GMV}(\Sigma(\theta')) - w_{GMV}(\Sigma(\theta))||^2}{H(\theta, \theta')} &\geq \frac{9\tau^2}{16p^2n}, \end{aligned}$$

where the last inequality is satisfied since  $|\theta|\tau/(p\sqrt{n}) \leq M/3$ . By applying this inequality and the result of Lemma S3.1 to Assouad's lemma, we complete the proof.  $\square$

Next, we give the proof of Lemma 3.3. For this proof we present Lemma S3.2.

**Lemma S3.2.** Suppose the notation of  $\mathcal{G}^{(2)}$  in (3) and assume  $2k\epsilon_{n,p}M^{-1} < 1$ . Let  $(\Sigma(\theta') - \Sigma(\theta))\Sigma(\theta)^{-1}\mathbf{1} = (x_1, \dots, x_p)$ . For  $i \leq r$  with  $\gamma_i(\theta') \neq \gamma_i(\theta)$ ,

$$x_i = (\gamma_i(\theta') - \gamma_i(\theta))k\epsilon_{n,p}(M^{-1} + \delta_i),$$

with

$$|\delta_i| \leq \frac{2k\epsilon_{n,p}}{M^2(1 - 2k\epsilon_{n,p}/M)}.$$

*Proof.* By the definition of the infinity norm and Theorem 2.3.4. in Golub and Van Loan (1996), we have

$$\begin{aligned} ||(\Sigma(\theta)^{-1} - M^{-1}I_p)\mathbf{1}||_\infty &\leq ||\Sigma(\theta)^{-1} - M^{-1}I_p||_\infty \\ &\leq \frac{1}{M^2} \frac{||\Sigma(\theta) - MI_p||_\infty}{1 - M^{-1}||\Sigma(\theta) - MI_p||_\infty}. \end{aligned}$$

Since  $M^{-1}||\Sigma(\theta) - MI_p||_\infty \leq 2k\epsilon_{n,p}M^{-1} < 1$ , we have

$$||(\Sigma(\theta)^{-1} - M^{-1}I_p)\mathbf{1}||_\infty \leq \frac{2k\epsilon_{n,p}}{M^2(1 - 2k\epsilon_{n,p}/M)}. \quad (\text{S12})$$

Next, we check  $x_i$  when  $i \leq r$ ,  $\gamma_i(\theta') = 1$  and  $\gamma_i(\theta) = 0$ . By the definition of  $\Sigma(\theta')$ , we have

$$\begin{aligned} x_i &= [\Sigma(\theta')]_i \Sigma(\theta)^{-1} \mathbf{1} \\ &= M^{-1}[\Sigma(\theta')]_i \mathbf{1} + [\Sigma(\theta')]_i ((\Sigma(\theta)^{-1} - M^{-1}I_p)\mathbf{1}) \\ &= M^{-1}k\epsilon_{n,p} + [\Sigma(\theta')]_i ((\Sigma(\theta)^{-1} - M^{-1}I_p)\mathbf{1}). \end{aligned}$$

By (S12),

$$\begin{aligned} |[\Sigma(\theta')]_i ((\Sigma(\theta)^{-1} - M^{-1}I_p)\mathbf{1})| &\leq ||[\Sigma(\theta')]_i||_1 ||(\Sigma(\theta)^{-1} - M^{-1}I_p)\mathbf{1}||_\infty \\ &\leq k\epsilon_{n,p} \frac{2k\epsilon_{n,p}}{M^2(1 - 2k\epsilon_{n,p}/M)}. \end{aligned}$$

Thus, we have

$$|x_i - M^{-1}k\epsilon_{n,p}| \leq k\epsilon_{n,p} \frac{2k\epsilon_{n,p}}{M^2(1 - 2k\epsilon_{n,p}/M)},$$

for  $i \leq r$  with  $\gamma_i(\theta') = 1$  and  $\gamma_i(\theta) = 0$ . Likewise, when  $\gamma_i(\theta') = 0$  and  $\gamma_i(\theta) = 1$ , we have

$$|x_i + M^{-1}k\epsilon_{n,p}| \leq k\epsilon_{n,p} \frac{2k\epsilon_{n,p}}{M^2(1 - 2k\epsilon_{n,p}/M)}.$$

Collecting these inequalities, we complete the proof. □

*Proof of Lemma 3.3.* We have

$$\frac{\Sigma(\theta)^{-1}\mathbf{1}}{\mathbf{1}^T \Sigma(\theta)^{-1}\mathbf{1}} - \frac{\Sigma(\theta')^{-1}\mathbf{1}}{\mathbf{1}^T \Sigma(\theta')^{-1}\mathbf{1}} = \frac{\Sigma(\theta')^{-1}}{\mathbf{1}^T \Sigma(\theta)^{-1}\mathbf{1}} (I_p - \frac{\mathbf{1}\mathbf{1}^T \Sigma(\theta')^{-1}}{\mathbf{1}^T \Sigma(\theta')^{-1}\mathbf{1}}) (\Sigma(\theta') - \Sigma(\theta)) \Sigma(\theta)^{-1}\mathbf{1},$$

and

$$\begin{aligned} &\left\| \frac{\Sigma(\theta)^{-1}\mathbf{1}}{\mathbf{1}^T \Sigma(\theta)^{-1}\mathbf{1}} - \frac{\Sigma(\theta')^{-1}\mathbf{1}}{\mathbf{1}^T \Sigma(\theta')^{-1}\mathbf{1}} \right\|_2 \\ &= \sup_{v: ||v||_2 \neq 0} \left[ \frac{v^T \Sigma(\theta')^{-1}}{||v||_2 \mathbf{1}^T \Sigma(\theta)^{-1}\mathbf{1}} (I_p - \frac{\mathbf{1}\mathbf{1}^T \Sigma(\theta')^{-1}}{\mathbf{1}^T \Sigma(\theta')^{-1}\mathbf{1}}) (\Sigma(\theta') - \Sigma(\theta)) \Sigma(\theta)^{-1}\mathbf{1} \right]. \end{aligned} \quad (\text{S13})$$

Define  $v_0 \in \mathbb{R}^p$  such that  $v_0^T \Sigma(\theta')^{-1} = (w_1, \dots, w_p)$  and

$$w_i = \begin{cases} \gamma_i(\theta') - \gamma_i(\theta), & \text{if } 1 \leq i \leq r, \\ \gamma_{i-r}(\theta) - \gamma_{i-r}(\theta'), & \text{if } r+1 \leq i \leq 2r, \\ 0, & \text{otherwise,} \end{cases}$$

which satisfies

$$(w_1, \dots, w_p)\mathbf{1} = 0. \quad (\text{S14})$$

Let  $(\Sigma(\theta') - \Sigma(\theta))\Sigma(\theta)^{-1}\mathbf{1} = (x_1, x_2, \dots, x_p)$ . When  $r < i \leq 2r$ ,  $x_i = 0$  by the definition of  $\Sigma(\theta)$  in  $\mathcal{G}^{(2)}$  and the fact that  $2r \leq p/2$ . Then, using Lemma S3.2, we have

$$\begin{aligned} (w_1, \dots, w_p)(\Sigma(\theta') - \Sigma(\theta))\Sigma(\theta)^{-1}\mathbf{1} &= \sum_{i=1}^p x_i w_i \\ &= H(\theta, \theta')k\epsilon_{n,p}(M^{-1} + \delta), \end{aligned}$$

with

$$|\delta| \leq \frac{2k\epsilon_{n,p}}{M^2(1 - 2k\epsilon_{n,p}/M)}.$$

Thus, we get

$$|(w_1, \dots, w_p)(\Sigma(\theta') - \Sigma(\theta))\Sigma(\theta)^{-1}\mathbf{1}| \geq k\epsilon_{n,p}H(\theta, \theta')(M^{-1} - \frac{2k\epsilon_{n,p}}{M^2(1 - 2k\epsilon_{n,p})}). \quad (\text{S15})$$

We also have

$$\begin{aligned} \|v_0\| &\leq \|\Sigma(\theta)^{-1}\| \|w\| \\ &\leq \sqrt{2H(\theta, \theta')/\lambda_{\min}(\Sigma(\theta))}. \end{aligned} \quad (\text{S16})$$

Collecting (S13), (S14), (S15) and (S16), we obtain

$$\begin{aligned} \left\| \frac{\Sigma(\theta)^{-1}\mathbf{1}}{\mathbf{1}^T \Sigma(\theta)^{-1}\mathbf{1}} - \frac{\Sigma(\theta')^{-1}\mathbf{1}}{\mathbf{1}^T \Sigma(\theta')^{-1}\mathbf{1}} \right\|_2 &\geq \frac{v_0^T \Sigma(\theta')^{-1}}{\|v_0\|_2 \mathbf{1}^T \Sigma(\theta)^{-1}\mathbf{1}} (I_p - \frac{\mathbf{1}\mathbf{1}^T \Sigma(\theta')^{-1}}{\mathbf{1}^T \Sigma(\theta')^{-1}\mathbf{1}})(\Sigma(\theta') - \Sigma(\theta))\Sigma(\theta)^{-1}\mathbf{1} \\ &\geq \frac{\sqrt{2H(\theta, \theta')\lambda_{\min}(\Sigma(\theta))}}{\mathbf{1}^T \Sigma(\theta)^{-1}\mathbf{1}} k\epsilon_{n,p}(M^{-1} - \frac{2k\epsilon_{n,p}}{M^2(1 - 2k\epsilon_{n,p})}) \\ &\geq \frac{\sqrt{2H(\theta, \theta')}}{p} k\epsilon_{n,p}(M^{-1} - \frac{2k\epsilon_{n,p}}{M^2(1 - 2k\epsilon_{n,p})}). \end{aligned}$$

Let  $\epsilon_{n,p} = (0.25(\log 2) \min(1, M_1) C_0^{-1})^{1/(1-q)} ((\log p)/n)^{1/2}$  and  $k = \max(\lfloor c_{n,p} \epsilon_{n,p}^{-q} \rfloor, 0)$ . Then, there exist a positive constant  $C_2$  such that

$$\min_{H(\gamma(\theta), \gamma(\theta')) \geq 1} \frac{\|w_{GMV}(\Sigma(\theta)) - w_{GMV}(\Sigma(\theta'))\|^2 r}{H(\gamma(\theta), \gamma(\theta'))} \frac{r}{2} \geq \frac{C_2 c_{n,p}^2}{p} \left( \frac{\log p}{n} \right)^{1-q},$$

for all sufficiently large  $n$ . By Lemma 6 in Cai et al. (2012),

$$\min_{1 \leq i \leq r} \|\bar{\mathbb{P}}_{i,0} \wedge \bar{\mathbb{P}}_{i,1}\| \geq C_3,$$

for a positive constant. Combining the two inequalities, we complete the proof.  $\square$

## References

- Cai, T. T., Zhou, H. H. et al. (2012). Optimal rates of convergence for sparse covariance matrix estimation, *The Annals of Statistics* **40**(5): 2389–2420.
- Golub, G. H. and Van Loan, C. F. (1996). Matrix computations. johns hopkins studies in the mathematical sciences.
- Lee, K., Lee, K. and Lee, J. (2021). Minimax analysis of the conditional mean linear operator under the bandable covariance structure, *unpublished manuscript* .
- Press, S. J. (2012). *Applied multivariate analysis: using Bayesian and frequentist methods of inference*, Courier Corporation.
